# Supplementary material for: SS-SFDA : Self-Supervised Source-Free Domain Adaptation for Road Segmentation in Hazardous Environments
Source: arXiv:2012.08939 source file (2021-03-25)
Supplement: Supplementary file 2 [file suppWeather.tex]

\begin{table}[H]
% \footnotesize
\label{tab:supp_datasets}
\centering
% \begin{center}
 \resizebox{\textwidth}{!}{
%\resizebox{\columnwidth}{!}{
\begin{tabular}{r c c c c}
\toprule
Dataset & Syn./Real & Weather & Time of Day & Image Size\\
\midrule
Rainy CityScapes \cite{halder2019physics}& Syn & Varying intensities (1mm - 200mm) of rain & Daytime & $512,1024$\\
Foggy CityScapes \cite{halder2019physics}& Syn & Varying intensities (750m - 30m) of fog & Daytime & $512,1024$\\
Foggy Zurich \cite{sakaridis2018model}& Real & Light and medium Fog & Daytime & $540,960$\\
Dark Zurich \cite{sakaridis2019guided}& Real & Clear & Twilight, Night &  $540,960$\\
Raincouver \cite{tung2017raincouver}& Real & Rain & Twilight, Night & $360,640$ \\
BDD \cite{yu2018bdd100k}& Real & Clear, Snow, Fog, Rain & Daytime, Twilight, Night & $720,1280$\\

\bottomrule
\end{tabular}

} %For resize box
% \caption{\textbf{List of datasets:} The second column categorizes the datasets as synthetic or real and the third, fourth and fifth columns describe the images contained in the dataset.}
% \vspace{-15pt}
% \end{center}
\end{table}
